# Supplementary material for: Moving Window Network Coding in Cooperative Multicast (v1)
Source: arXiv:1209.3827 source file (2012-09-18)
Supplement: Supplementary file 1 [file appendix.tex]

\begin{appendices}

\setcounter{equation}{0}

\section{Proof of Theorem 1}\label{sec:appendix}

Remember the available stations with maximum residual profit are
added in turn. Several relations regarding residual profit of an
added relay or between two different selections are going to be
established. Lemma 1,2 show that to add or to remove a relay chance
only the residual profit part. Lemma 3 compares the profit
difference of two different selections. Lemma 4 reveals a property
of the greedy selection relative an arbitrary selection.

\begin{lemma}\label{lemma:appendix1}
Let $S=(\beta)$, and let
$S'=(\beta\oplus j)$, where $j\not\in \beta$ is a candidate
relay. Then $C_{S}(j)=C(S^\prime)-C(S),W_{S}(j)=1$.
\end{lemma}

\begin{proof}
By definition, we have
\begin{equation}
\begin{split}
C_S(j)&=\sum_{j\in \mathcal{E}}C_S(f^\prime (j),j) \\
      & = \sum_{j\in \mathcal{E}}(C(f^\prime
(j),j)-C(f(j),j))\nonumber\\
 & =C(S')-C(S)
\end{split}
\end{equation}
Since $b\not\in S$, $W_S(b)=W(b)=1$.
\end{proof}

\begin{lemma}\label{lemma:appendix2}
Let $S=(\beta)$, and let
$S^\prime=(\beta\ominus j)$, where $j$ is a relay in $S$. Then $C_{S}(\ominus j)=C(S^\prime)-C(S),W_{S}(\ominus j)=1$.
\end{lemma}

The proof of Lemma~\ref{lemma:appendix2} is similar to the proof of Lemma \ref{lemma:appendix1}.

\begin{lemma} For any two selections
$S = (\beta)$ and $S^\prime=(\beta^\prime)$,
$C_S(S^\prime)=C(S^\prime)-C(S)$.
\end{lemma}

\begin{proof} By definition, $C_S(S^\prime)=\sum_j
C_S(f^\prime (j),j)$ is the summation over all end receivers.
Therefore, there exists two sequences of relays $R_+$ and $R_-$ such that
$S^\prime=S\oplus R_+\ominus R_-$. By Lemma 1,2, we have the
conclusion.
\end{proof}

\begin{lemma}  Let $S$ be a selection, then the
following result is held for every $k$($0<k<K$):
\begin{eqnarray}
C(S_{k+1})-C(S_{k})=\frac{C_k(j_k)}{W_k(j_k)}\ge
\frac{C_k(S)}{W_k(S)}=\frac{C(S)-C(S_k)}{W_k(S)}
\end{eqnarray}
\end{lemma}

\begin{proof} As specified, adding one relay
increases the cost by 1, thus $W_k(j_k)=1$, so the first equation
holds. To prove the second inequality, let the average residual
density of $S$ with respect to $S_k$ be $d=\frac{C_k(S)}{W_k(S)}$.
At least one relay in $S$, say $i$, has a density greater than $d$,  which is true for addition to $S_i$ in the first $K-2$ rounds. Since
the relay with the largest residual density is added, its density
must be no less than $i$. The last equality follows directly from
Lemma 3.
\end{proof}

Finally, we can prove Theorem 1 based on Lemma to Lemma . 

\begin{proof} Lemma 4 implies that for any selection
$S$, say the globally optimal selection $S$, the augmentation every
iteration is at least $\frac{1}{W_i(S)}$ of the difference with
$C(S)$. If the relays greedily in the first $j$ rounds are really in
the globally optimal selection, $W_i(S)=K-1-i$ and it can guarantee
to increase no less than $\frac{k}{K-1}P(S)$ just in the $k$th rounds.
However, we can not predict $k$, so in the worst case, $k\equiv
K-1$. So the worst bound is derived. Besides, in the aggregate,
$K-1$ rounds with each round pick one relay from $N_S$ candidates,
so the time complexity is $O(N_S\times (K-1)$.
\end{proof}

\end{appendices}
